# Supplementary material for: Generating Maximal Configurations and Their Variants Using Code Metrics
Source: arXiv:2401.07898 source file (2024-01-15)
Supplement: Supplementary file 1 [file additionaldata.tex]

\begin{comment}
\begin{table*}
\begin{footnotesize}
    \begin{tabular}{c|r|r|r|r|r|r|r|r|r|r|r|r|r|r|r} \toprule
          &  & \multicolumn{7}{c|}{MaxSAT Variants (Scores \& Time)} &  \multicolumn{7}{c|}{Presence Condition Fuzzing (Average Scores \& Time (secs))} \\ \cline{3-16}
         {\bf Comp.} & {\bf \# UPC} & {\bf \#} & {\bf Max} & {\bf Min} & {\bf Med.} & {\bf Mean} & {\bf Std.} & {\bf Time} & {\bf \#} & {\bf Max} & {\bf Min} & {\bf Med.} & {\bf Mean} & {\bf Std.} & {\bf Time}\\ \hline
awk & 65 & 542 & 66 & 1 & 26.0 & 23.90 & 16.77 & & 2272.8 & 55.6 & 0.0 & 18.8 & 23.27 & 16.86 & \\
cmp & 62 & 396 & 74 & 25 & 29.0 & 32.88 & 12.01 & & 2916.6 & 62.6 & 0.0 & 23.0 & 26.44 & 17.21 & \\
diff & 68 & 584 & 73 & 1 & 25.0 & 24.03 & 18.00 & & 2129.0 & 57.0 & 0.0 & 17.6 & 23.19 & 17.59 & \\
ed & 63 & 1183 & 65 & 1 & 25.0 & 23.26 & 8.89 & & 2233.2 & 53.0 & 0.0 & 18.8 & 22.80 & 16.06   \\
patch\_bbox & 65 & 772 & 71 & 2 & 22.0 & 15.78 & 14.98 & & 2042.2 & 58.0 & 0.0 & 17.6 & 23.20 & 17.72 & \\
patch\_toybox & 63 & 1183 & 65 & 1 & 25.0 & 23.26 & 8.89 & & 2169.6 & 56.8 & 0.0 & 18.2 & 23.19   &16.99 & \\
patch & 65 & 772 & 71 & 2 & 22.0 & 15.78 & 14.98 & & 2212.8 & 57.6 & 0.0 & 18.6 & 22.56 & 16.15 & \\
sed & 65 & 1289 & 71 & 1 & 27.0 & 25.31 & 9.45 & & 2273.0 & 56.2 & 0.0 & 19.0 & 23.50 & 16.83 & \\
         \bottomrule
    \end{tabular}
    \end{footnotesize}
    \caption{Comparison of configuration generation approaches for the BusyBox {\em editors} subsystem in terms of the number of generated configurations (\#), maximum, minimum, median, and standard deviation of scores for the LCU metric. UPC denotes the number of unique presence conditions. Fuzzing results are the averages of 5 runs. The fuzzing seed consists of all presence conditions turned off. Number of cycles=3.}
    \label{tab:statcmpeditors}
\end{table*}

\begin{table*}
\begin{footnotesize}
    \begin{tabular}{c|r|r|r|r|r|r|r|r|r|r|r|r|r|r|r} \toprule
          &  & \multicolumn{7}{c|}{MaxSAT Variants (Scores \& Time)} &  \multicolumn{7}{c|}{Presence Condition Fuzzing (Average Scores \& Time (secs))} \\ \cline{3-16}
         {\bf Comp.} & {\bf \# UPC} & {\bf \#} & {\bf Max} & {\bf Min} & {\bf Med.} & {\bf Mean} & {\bf Std.} & {\bf Time} & {\bf \#} & {\bf Max} & {\bf Min} & {\bf Med.} & {\bf Mean} & {\bf Std.} & {\bf Time}\\ \hline
awk & 65 & 542 & 66 & 1 & 26.0 & 23.90 & 16.77 & & 4262.0 & 67.2 & 0.0 & 45.8 & 38.81 & 21.31 & \\
cmp & 62 & 396 & 74 & 25 & 29.0 & 32.88 & 12.01 & & 7178.6 & 71.4 & 0.0 & 43.4 & 40.23 & 19.35  & \\
diff & 68 & 584 & 73 & 1 & 25.0 & 24.03 & 18.00 & & 3976.4 & 71.0 & 0.0 & 48.8 & 40.60 & 22.91 & \\
ed & 63 & 1183 & 65 & 1 & 25.0 & 23.26 & 8.89 & & 4234.4 & 66.8 & 0.0 & 46.0 & 38.64 & 20.84 & \\
patch\_bbox & 65 & 772 & 71 & 2 & 22.0 & 15.78 & 14.98 & & 4465.2 & 70.2 & 0.0 & 46.0 & 39.24 & 21.67 & \\
patch\_toybox & 63 & 1183 & 65 & 1 & 25.0 & 23.26 & 8.89 & & 4153.6 & 65.4 & 0.0 & 45.8 & 38.07 & 20.42 & \\
patch & 65 & 772 & 71 & 2 & 22.0 & 15.78 & 14.98 & & 4126.8 & 70.0 & 0.0 & 47.8 & 40.26 & 22.11 & \\
sed & 65 & 1289 & 71 & 1 & 27.0 & 25.31 & 9.45 & & 4076.6 & 70.6 & 0.0 & 49.0 & 40.52 & 22.73 & \\
         \bottomrule
    \end{tabular}
    \end{footnotesize}
    \caption{Comparison of configuration generation approaches for the BusyBox {\em editors} subsystem in terms of the number of generated configurations (\#), maximum, minimum, median, and standard deviation of scores for the LCU metric. UPC denotes the number of unique presence conditions. Fuzzing results are the averages of 5 runs. The fuzzing seed consists of all presence conditions turned off. Number of cycles=10.}
    \label{tab:statcmpeditors}
\end{table*}

\begin{table*}
\begin{footnotesize}
    \begin{tabular}{c|r|r|r|r|r|r|r|r|r|r|r|r|r|r|r} \toprule
          &  & \multicolumn{7}{c|}{MaxSAT Variants (Scores \& Time)} &  \multicolumn{7}{c|}{Presence Condition Fuzzing (Average Scores \& Time (secs))} \\ \cline{3-16}
         {\bf Comp.} & {\bf \# UPC} & {\bf \#} & {\bf Max} & {\bf Min} & {\bf Med.} & {\bf Mean} & {\bf Std.} & {\bf Time} & {\bf \#} & {\bf Max} & {\bf Min} & {\bf Med.} & {\bf Mean} & {\bf Std.} & {\bf Time}\\ \hline
awk & 65 & 542 & 66 & 1 & 26.0 & 23.90 & 16.77 & & 5737.8 & 67.8 & 0.0 & 54.4 & 45.42 & 21.25 & \\
cmp & 62 & 396 & 74 & 25 & 29.0 & 32.88 & 12.01 & & 8615.6 & 72.0 & 0.0 & 52.4 & 45.86 & 20.35  & \\
diff & 68 & 584 & 73 & 1 & 25.0 & 24.03 & 18.00 & & 5320.6 & 72.0 & 0.0 & 59.2 & 48.12 & 23.31 & \\
ed & 63 & 1183 & 65 & 1 & 25.0 & 23.26 & 8.89 & & 5431.4 & 65.4 & 0.0 & 51.5 & 43.00 & 20.25 & \\
patch\_bbox & 65 & 772 & 71 & 2 & 22.0 & 15.78 & 14.98 & & 5165.4 & 70.4 & 0.0 & 54.4 & 45.60 & 22.12 & \\
patch\_toybox & 63 & 1183 & 65 & 1 & 25.0 & 23.26 & 8.89 & & 5487.2 & 65.4 & 0.0 & 51.6 & 43.02 & 20.15 & \\
patch & 65 & 772 & 71 & 2 & 22.0 & 15.78 & 14.98 & & 6133.6 & 70.2 & 0.0 & 51.8 & 43.93 & 21.55 & \\
sed & 65 & 1289 & 71 & 1 & 27.0 & 25.31 & 9.45 & & 5940.6 & 70.0 & 0.0 & 54.4 & 46.00 & 21.17 & \\
         \bottomrule
    \end{tabular}
    \end{footnotesize}
    \caption{Comparison of configuration generation approaches for the BusyBox {\em editors} subsystem in terms of the number of generated configurations (\#), maximum, minimum, median, and standard deviation of scores for the LCU metric. UPC denotes the number of unique presence conditions. Fuzzing results are the averages of 5 runs. The fuzzing seed consists of all presence conditions turned off. Number of cycles=20.}
    \label{tab:statcmpeditors}
\end{table*}
\end{comment}
